# Supplementary material for: Striped spin liquid crystal ground state instability of kagome antiferromagnets
Source: arXiv:1210.1585 ancillary file (2012-10-04)
Supplement: Supplementary file 1 [file kagome-supplementary-arXiv-v1.pdf]

# SUPPLEMENTARY INFORMATION: $Z_2$ STRIPED SPIN LIQUID GROUND STATE OF KAGOME ANTIFERROMAGNETS

## S-I. THE MEAN FIELD THEORY

To find the BCS pairing functions, we begin with the mean field Hamiltonian in its Nambou-spinor form:

$$H_{m.f.} = \frac{3J}{8}\sum_{ij} J_{ij}\left[\frac{1}{4}\mathrm{tr}\mathbf{U}_{ij}^{\dagger}\cdot\mathbf{U}_{ij} - \hat{\psi}_i^{\dagger}\cdot\mathbf{U}_{ij}\cdot\hat{\psi}_j\right] + \sum_i \vec{a}_i\cdot\hat{\psi}_i^{\dagger}\cdot\vec{\tau}\cdot\hat{\psi}_i\Big] \quad (1)$$

where $\hat{\psi}_i^{\dagger} = (\hat{f}_{i\uparrow}^{\dagger}, \hat{f}_{i\downarrow})$ is a Nambou spinor, the $2\times 2$ matrix $\mathbf{U}_{ij}$ contains the hopping and pairing mean fields $\chi_{ij}$ and $\Delta_{ij}$

$$\mathbf{U}_{ij} = \begin{pmatrix} \chi_{ij}^{*} & -\Delta_{ij} \\ -\Delta_{ij}^{*} & -\chi_{ij} \end{pmatrix}, \quad (2)$$

defined through

$$\langle \hat{f}_{i\alpha}^{\dagger}\hat{f}_{j\beta}\rangle = \frac{1}{2}\chi_{ij}\delta_{\alpha\beta}, \quad \langle \hat{f}_{i\alpha}\hat{f}_{j\beta}\rangle = \frac{1}{2}\Delta_{ij}\epsilon_{\alpha\beta}, \quad (3)$$

and $\vec{a}_i$ are Lagrange multipliers responsible for imposing the constraint of one particle per site. Here $U_{ij} = U_{ji}^{\dagger}$ for $\chi_{ij} = \chi_{ji}^{*}$, $\Delta_{ij} = \Delta_{ji}$.

This Hamiltonian has the mentioned local $SU(2)$ symmetry. To see it, consider rotating the Nambou spinor by an $SU(2)$ matrix $\mathbf{G}_i$ so that $\psi_i \to \mathbf{G}_i\cdot\psi_i$. The Hamiltonain is then invariant provided we send $\mathbf{U}_{ij} \to \mathbf{G}_i\cdot\mathbf{U}_{ij}\cdot\mathbf{G}_i^{\dagger}$ and $\vec{a}_i\cdot\tau \to \mathbf{G}_i\cdot(\vec{a}_i\cdot\tau)\cdot\mathbf{G}_i^{\dagger}$. This invariance complicates the determination of the lowest energy mean field state and the interpretation of the results because of the immense redundancy in our choice of mean fields $\mathbf{U}_{ij}$, $\vec{a}_i$. If $\mathbf{U}_{ij}$, $\vec{a}_i$ is the lowest energy mean field configuration, then so is any gauge transformed configuration.

Now, Ref. 1 provides us with a representation of the space group generated by the group elements $G_1T_1, G_2T_2, G_RR, G_\sigma\sigma$ where $T_1$, $T_2$ are translations by a unit cell in the Bravais lattice directions $\vec{a}_1$, $\vec{a}_2$ respectively, $R$ is a $\pi/3$ rotation about the center of a hexagon, $\sigma$ is a mirror reflection in the plane of the lattice and $G_1$, $G_2$, etc., are gauge transformations that must follow these space group transformations. A general symmetry transformation in the group is then given by

$$D(g_i) = (G_1T_1)^m(G_2T_2)^n(G_RR)^{\ell}(G_\sigma\sigma)^p \quad (4)$$

where $m$ and $n$ are any integers (negative means translate the other way), $\ell \in \{0, \ldots, 5\}$ label the six possible $\pi/3$ rotations, $p \in \{0, 1\}$ and $g_i$ is an abstract symbol labeling the space group transformation represented by $D(g_i)$. The group then has multiplication table

$$D(g_i)D(g_j) = \mathcal{G}D(g_i g_j) \tag{5}$$

where $\mathcal{G} = \pm 1$ is an allowed additional phase altering the usual group multiplication table due to the identification of $D(g_i)$ and $-D(g_i)$ as the same transformation when we study wave functions $\psi$ and $-\psi$ that are physically equivalent. This additional phase makes this representation of the space group a "projective" representation similar to projective representations of groups in quantum mechanics[Hamermesh]. According to Ref. 1 there are at least 14 of these representations that are useful in constructing symmetry distinct wave functions on the kagome lattice.

Starting from one of these representations, we construct matrices $\mathbf{U}_{ij}$ that characterize a given mean field Hamiltonian by starting from one bond $\mathbf{U}_{12}$ and performing symmetry transformations

$$U_{g_i(1)g_i(2)} = D(g_i)\mathbf{U}_{12}D^{-1}(g_i), \tag{6}$$

where the bond 12 is mapped to $g_i(1)g_i(2)$ by the space group transformation $g_i$, until matrices $U_{ij}$ of all related bonds in the unit cell are found. For example, if bond 23 is related to 12 by the rotation $R$ then

$$U_{23} = \mathbf{G}_R(2) \cdot U_{12} \cdot \mathbf{G}_R^\dagger(2). \tag{7}$$

We performed this for four types of bonds necessary to construct the distinct wave functions outlined in Ref. 1: nearest neighbor, second neighbor and two types of third neighbors.

## S-II. DIAGONALIZATION OF THE MEAN FIELD HAMILTONIAN

To diagonalize our mean field Hamiltonian, let's begin by simplifying notation. Let $h_{ij} = -\frac{3}{8}J_{ij}U_{ij}$, for $i \neq j$, and $h_{ii} = \vec{a}_i \cdot \vec{\tau}$. Furthermore, let us organize the spinor variables into the vector

$$\Psi^\dagger = \left(\hat{f}^\dagger_{1\uparrow}, \ldots, \hat{f}^\dagger_{Ns\uparrow}, \hat{f}_{1\downarrow}, \ldots, \hat{f}_{Ns\downarrow}\right) \equiv \left(\hat{f}^\dagger_\uparrow, \hat{f}_\downarrow\right) \tag{8}$$

where we have adopted a simplified two-component notation in the last step that involves just dropping indices. Using this notation, the fermion part of the Hamiltonian becomes

$$H_{fermion} = \hat{\Psi}^{\dagger} \cdot \mathbf{h} \cdot \hat{\Psi} = (\hat{f}_{\uparrow}^{\dagger}, \hat{f}_{\downarrow}) \begin{pmatrix} -\chi^* & \Delta \\ \Delta^* & \chi \end{pmatrix} \begin{pmatrix} \hat{f}_{\uparrow} \\ \hat{f}_{\downarrow}^{\dagger} \end{pmatrix} \tag{9}$$

where we have also adopted a two-component notation for $\mathbf{h}$ after setting $\chi_{ii} = -a_{3i}$ and $\Delta_{ii} = a_{1i} - ia_{2i}$ and then dropping indices. To diagonalize this Hamiltonian, we perform the linear transformation

$$\hat{\Psi} = \mathbf{T} \cdot \hat{\Gamma} = \mathbf{T} \cdot \begin{pmatrix} \gamma_1 \\ \gamma_2^{\dagger} \end{pmatrix} \tag{10}$$

For this to be a canonical transformation, we must have $\mathbf{T}^{\dagger}\mathbf{T} = \mathbf{T}\mathbf{T}^{\dagger} = \mathbf{I}$. Namely, $\mathbf{T}$ must be a unitary matrix. Since $\mathbf{h}$ is a Hermitian matrix, we can then always find a transformation $T$ that diagonalizes the Hamiltonian by solving $\mathbf{h} \cdot \mathbf{T} = \mathbf{T} \cdot \epsilon$ so that the columns of $T$ are the eigenvectors of $\mathbf{h}$.

It us useful to consider this diagonalization more concretely using our $2 \times 2$ simplified notation. Let

$$\mathbf{T} = \begin{pmatrix} U_1 & V_2 \\ V_1 & U_2 \end{pmatrix}. \tag{11}$$

Then the linear transformation takes the form

$$\mathbf{f}_{\uparrow} = \mathbf{U}_1 \cdot \gamma_1 + \mathbf{V}_2 \cdot \gamma_2^{\dagger}, \quad \mathbf{f}_{\downarrow}^{\dagger} = \mathbf{V}_1 \cdot \gamma_1 + \mathbf{U}_2 \cdot \gamma_2^{\dagger} \tag{12}$$

and its inverse is

$$\gamma_1 = \mathbf{U}_1^{\dagger} \cdot \mathbf{f}_{\uparrow} + \mathbf{V}_1^{\dagger} \cdot \mathbf{f}_{\downarrow}^{\dagger}, \quad \gamma_2^{\dagger} = \mathbf{V}_2^{\dagger} \cdot \mathbf{f}_{\uparrow} + \mathbf{U}_2^{\dagger} \cdot \mathbf{f}_{\downarrow}^{\dagger} \tag{13}$$

so that the annihilation operator becomes $\gamma_2 = \mathbf{U}_2^{T} \cdot \mathbf{f}_{\downarrow} + \mathbf{V}_2^{T} \cdot \mathbf{f}_{\uparrow}^{\dagger}$ (used below in the construction of the ground state). From $\mathbf{T}^{\dagger} \cdot \mathbf{T} = \mathbf{I}$, the sub-matrices must obey

$$\mathbf{U}_1^{\dagger} \cdot \mathbf{U}_1 + \mathbf{V}_1^{\dagger} \cdot \mathbf{V}_1 = \mathbf{I}, \quad \mathbf{U}_1^{\dagger} \cdot \mathbf{V}_2 + \mathbf{V}_1^{\dagger} \cdot \mathbf{U}_2 = 0, \quad \mathbf{V}_2^{\dagger} \cdot \mathbf{U}_1 + \mathbf{U}_2^{\dagger} \cdot \mathbf{V}_1 = 0, \quad \mathbf{V}_2^{\dagger} \cdot \mathbf{V}_2 + \mathbf{U}_2^{\dagger} \cdot \mathbf{U}_2 = \mathbf{I} \tag{14}$$

and further $\mathbf{T} \cdot \mathbf{T}^{\dagger} = \mathbf{I}$ imposes

$$\mathbf{U}_1 \cdot \mathbf{U}_1^{\dagger} + \mathbf{V}_2 \cdot \mathbf{V}_2^{\dagger} = \mathbf{I}, \quad \mathbf{U}_1 \cdot \mathbf{V}_1^{\dagger} + \mathbf{V}_2 \cdot \mathbf{U}_2^{\dagger} = 0, \quad \mathbf{V}_1 \cdot \mathbf{U}_1^{\dagger} + \mathbf{U}_2 \cdot \mathbf{V}_2^{\dagger} = 0, \quad \mathbf{V}_1 \cdot \mathbf{V}_1^{\dagger} + \mathbf{U}_2 \cdot \mathbf{U}_2^{\dagger} = \mathbf{I} \tag{15}$$

We shall find these relations useful below in the construction of the ground state.

Finally, in two-component form, the eigenvalue equation we are interested in solving is

$$\begin{pmatrix} -\chi^* & \Delta \\ \Delta^* & \chi \end{pmatrix} \begin{pmatrix} U_{1m} \\ V_{1m} \end{pmatrix} = \epsilon_{1m} \begin{pmatrix} U_{1m} \\ V_{1m} \end{pmatrix}, \quad \begin{pmatrix} -\chi^* & \Delta \\ \Delta^* & \chi \end{pmatrix} \begin{pmatrix} V_{2m} \\ U_{2m} \end{pmatrix} = -\epsilon_{2m} \begin{pmatrix} V_{2m} \\ U_{2\bar{m}} \end{pmatrix} \tag{16}$$

where the sign of the eigenvalues were chosen so that they correspond to positive energies (can we prove this?). The eigenvalues of $\mathbf{h}$ occur in pairs of opposite signs because of time-reversal symmetry (can we prove this?). In addition, the eigenvectors each have an overall phase ambiguity in that

$$\begin{pmatrix} U_{1m} \\ V_{1m} \end{pmatrix} \to e^{i\phi_{1m}} \begin{pmatrix} U_{1m} \\ V_{1m} \end{pmatrix}, \quad \begin{pmatrix} V_{2m} \\ U_{2m} \end{pmatrix} \to e^{i\phi_{2m}} \begin{pmatrix} V_{2m} \\ U_{2m} \end{pmatrix} \tag{17}$$

We shall see below that the ground state wave function is independent of these phases.

### Ground state wave function

The ground state wave function, the empty state of $\gamma$-fermions is determined by the "pair wave function" $\phi_{ij}$ through

$$|\Omega\rangle = \prod_{ij} \left(1 + \phi_{ij} f_{i\uparrow}^\dagger f_{j\downarrow}^\dagger\right)|0\rangle = e^{\sum_{ij} \phi_{ij} f_{i\uparrow}^\dagger f_{j\downarrow}^\dagger}|0\rangle = e^{\mathbf{f}_\uparrow^\dagger \cdot \phi \cdot \mathbf{f}_\downarrow^\dagger}|0\rangle \tag{18}$$

where $|0\rangle$ is the unnormalized empty state of $f$-fermions and we see that $\phi_{ij} = -\phi_{ji}$. To find $\phi_{ij}$ we start from $\gamma_1|\Omega\rangle = 0$ and $\gamma_2|\Omega\rangle = 0$ and expand the exponential in the above expression. The first of these equations is then

$$\left(\mathbf{U}_1^\dagger \cdot \mathbf{f}_\uparrow + \mathbf{V}_1^\dagger \cdot \mathbf{f}_\downarrow^\dagger\right)\left[1 + \mathbf{f}_\uparrow^\dagger \cdot \phi \cdot \mathbf{f}_\downarrow^\dagger + \frac{1}{2}\left(\mathbf{f}_\uparrow^\dagger \cdot \phi \cdot \mathbf{f}_\downarrow^\dagger\right)^2 + \dots\right]|0\rangle \tag{19}$$

This expansion is then readily reorganized as a sum in groups of odd numbers of $f$-fermions. The one $f$-fermion contribution to the sum is then

$$V_1^\dagger \cdot \mathbf{f}_\downarrow^\dagger|0\rangle + \mathbf{U}_1^\dagger \cdot \mathbf{f}_\uparrow\left(\mathbf{f}_\uparrow^\dagger \cdot \phi \cdot \mathbf{f}_\downarrow^\dagger\right)|0\rangle \tag{20}$$

The second term only has finite contributions when we create and annihilate an $f_\uparrow$-fermion on the same site. Hence the one-fermion contribution simplifies to

$$V_1^\dagger \cdot \mathbf{f}_\downarrow^\dagger|0\rangle + \mathbf{U}_1^\dagger \cdot \phi \cdot \mathbf{f}_\downarrow^\dagger|0\rangle \tag{21}$$

So that choosing

$$\phi = -\mathbf{U}_1^{\dagger -1} \cdot \mathbf{V}_1^{\dagger} \tag{22}$$

will cause this contribution to vanish. To see if this choice holds to all orders in the sum, consider the $2k+1$-fermion contribution

$$\frac{1}{k!} V_1^{\dagger} \cdot \mathbf{f}_{\downarrow}^{\dagger} (\mathbf{f}_{\uparrow}^{\dagger} \cdot \phi \cdot \mathbf{f}_{\downarrow}^{\dagger})^k |0\rangle + \frac{1}{(k+1)!} \mathbf{U}_1^{\dagger} \cdot \mathbf{f}_{\uparrow} (\mathbf{f}_{\uparrow}^{\dagger} \cdot \phi \cdot \mathbf{f}_{\downarrow}^{\dagger})^{k+1} |0\rangle \tag{23}$$

Again, the second term vanishes unless we annihilate an $f_{\uparrow}$-fermion that was created in one of the $k+1$ possible places. Hence, this contribution simplifies to

$$\frac{1}{k!} V_1^{\dagger} \cdot \mathbf{f}_{\downarrow}^{\dagger} (\mathbf{f}_{\uparrow}^{\dagger} \cdot \phi \cdot \mathbf{f}_{\downarrow}^{\dagger})^k |0\rangle + \frac{1}{k!} \mathbf{U}_1^{\dagger} \cdot \phi \cdot \mathbf{f}_{\downarrow}^{\dagger} (\mathbf{f}_{\uparrow}^{\dagger} \cdot \phi \cdot \mathbf{f}_{\downarrow}^{\dagger})^k |0\rangle \tag{24}$$

and therefore also vanishes when we set $\phi = -\mathbf{U}_1^{\dagger -1} \cdot \mathbf{V}_1^{\dagger}$. So indeed Eq. (22) holds to all orders.

Following the same logic but starting from $\gamma_2|\Omega\rangle = 0$ leads to $\phi^T = \mathbf{U}_2^{T-1} \cdot \mathbf{V}_2^T$. Hence we require

$$\phi = -\mathbf{U}_1^{\dagger -1} \cdot \mathbf{V}_1^{\dagger} = \mathbf{V}_2 \cdot \mathbf{U}_2^{-1}, \tag{25}$$

or $\mathbf{U}_1^{\dagger} \cdot \mathbf{V}_2 + \mathbf{V}_1^{\dagger} \cdot \mathbf{U}_2 = 0$, for $|\Omega\rangle$ to be the empty state of $\gamma$-fermions. But this requirement is just one of those found in Eq. (14). So we may determine $\phi$ from Eq. (25) for any solution of the diagonalization problem, including those of Ref. 1.

Finally we note that changing the phase of the eigenvectors following Eq. (17) does not change $\phi$. Under this transformation, the $m$th row of $\mathbf{V}_1^{\dagger}$ picks up a phase factor $e^{-i\phi_{1m}}$ while the $m$th column of $\mathbf{U}_1^{\dagger -1}$ picks up a phase factor $e^{i\phi_{1m}}$ so that they cancel upon multiplication in Eq. (25). A similar arguments holds for the second form of $\phi$ found in Eq. (25).

## Fixing Lagrange multipliers

The Lagrange multipliers $a_1$, $a_2$ and $a_3$, which are the same on every site for the Z2 PSGs outlined in Lu, Ran and Lee, are determined by

$$\langle\Omega|\Psi^{\dagger} \cdot \tau \cdot \Psi|\Omega\rangle = 0 \tag{26}$$

where here we define the $2N \times 2N$ Pauli matrices to be

$$\tau_x = \begin{pmatrix} 0 & \mathbf{I} \\ \mathbf{I} & 0 \end{pmatrix}, \quad \tau_y = \begin{pmatrix} 0 & -i\mathbf{I} \\ i\mathbf{I} & 0 \end{pmatrix}, \quad \tau_z = \begin{pmatrix} \mathbf{I} & 0 \\ 0 & -\mathbf{I} \end{pmatrix}, \tag{27}$$

Hence these imply

$$\tau_x: \quad \mathrm{Tr}\left[U_2^\dagger \cdot V_2 + V_2^\dagger \cdot U_2\right] = 0, \quad \tau_y: \quad \mathrm{Tr}\left[U_2^\dagger \cdot V_2 - V_2^\dagger \cdot U_2\right] = 0, \quad \tau_z: \quad \mathrm{Tr}\left[U_2^\dagger \cdot U_2 - V_2^\dagger \cdot V_2\right] = 0, \tag{28}$$

If $T$ is real then the $\tau_y$ case is always obeyed. The other two cases are then all that is necessary to fix the constraints correctly.

### Time reversal invariance

Under the time reversal transformation $\mathcal{T} = -i\tau_2 K$ where $\tau_2$ is the $2N \times 2N$ Pauli matrix defined above and $K$ the complex conjugation operator, the matrix $T$ transforms to $\mathcal{T}\mathbf{T}\mathcal{T}^{-1}$. If this transformation is an invariance for $\mathbf{T}$ then we discover $U_1 = U_2^*$ and $V_1 = -V_2^*$. If we Choose $U_2 = U$ and $V_2 = V$, we then find the usual Bogoliubov version of the transformation:

$$\gamma_\uparrow = U^T \cdot f_\uparrow - V^T \cdot f_\downarrow^\dagger, \quad \gamma_\downarrow = U^T \cdot f_\downarrow + V^T \cdot f_\uparrow^\dagger \tag{29}$$

In addition we find that the pairing amplitude matrix $\phi$ is symmetric:

$$\phi^T = -\mathbf{V}_1 * \cdot \mathbf{U}_1^{*-1} = \mathbf{V}_2 \cdot \mathbf{U}_2^{-1} = \phi \tag{30}$$

## S-III. PAIRING MATRIX OF OUR LOWEST OPTIMIZED STATE

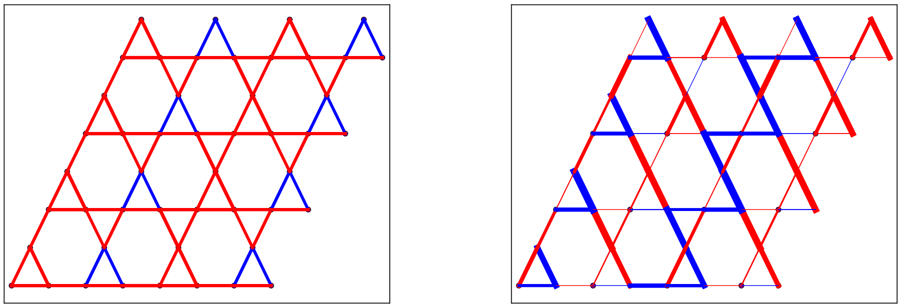

(a) (b)

FIG. 1. Values of the pairing matrix for our optimal state. (a) $\phi(\vec{r}_{i\uparrow}, \vec{r}_{j\downarrow})$. (b): Values of $|\phi| - \overline{|\phi|}$. The color here indicates the sign and the linewidth measures the magnitude.

## S-IV. TRANSFORMATIONS OF THE $w$-MONOPOLE OPERATOR

Constructing the 6 dimensional vector monopole operator

$$(\mathrm{Re}\,\hat{w}_x, \mathrm{Re}\,\hat{w}_y, \mathrm{Re}\,\hat{w}_z, \mathrm{Im}\,\hat{w}_x, \mathrm{Im}\,\hat{w}_y, \mathrm{Im}\,\hat{w}_z)^T, \tag{31}$$

we find it transforms under the 6 fold rotation $R(R_{\pi/3})$, mirror $R(\mathcal{R}_y)$, and translation $R(T_{\mathbf{a}_1})$ symmetries through the matrices:

$$\frac{1}{2}\begin{pmatrix} 0 & -1 & 0 & 0 & \sqrt{3} & 0 \\ 0 & 0 & 1 & 0 & 0 & \sqrt{3} \\ 1 & 0 & 0 & -\sqrt{3} & 0 & 0 \\ 0 & -\sqrt{3} & 0 & 0 & -1 & 0 \\ 0 & 0 & \sqrt{3} & 0 & 0 & 1 \\ \sqrt{3} & 0 & 0 & 1 & 0 & 0 \end{pmatrix}, \begin{pmatrix} 0 & 0 & 1 & 0 & 0 & 0 \\ 0 & -1 & 0 & 0 & 0 & 0 \\ 1 & 0 & 0 & 0 & 0 & 0 \\ 0 & 0 & 0 & 0 & 0 & -1 \\ 0 & 0 & 0 & 0 & 1 & 0 \\ 0 & 0 & 0 & -1 & 0 & 0 \end{pmatrix}, \begin{pmatrix} -1 & 0 & 0 & 0 & 0 & 0 \\ 0 & 1 & 0 & 0 & 0 & 0 \\ 0 & 0 & -1 & 0 & 0 & 0 \\ 0 & 0 & 0 & -1 & 0 & 0 \\ 0 & 0 & 0 & 0 & 1 & 0 \\ 0 & 0 & 0 & 0 & 0 & -1 \end{pmatrix}, \tag{32}$$

which follow directly from Ref. 2 after taking the parameter $n_R = 2$ that was left undetermined by them but suggested to take this value based on some numerical results. By taking the trace of these matrices to generate the characters of this representation and comparing them to the character table in Ref. 2 shows that it is composed of the $F_1$ and $F_2$ irriducible representations.

---


[1] Y.-m. Lu, Y. Ran, and P. Lee, Physical Review B, **83**, 12 (2011), ISSN 1098-0121, arXiv:1104.1432.

[2] M. Hermele, Y. Ran, P. Lee, and X.-G. Wen, Physical Review B, **77**, 224413 (2008), ISSN 1098-0121.
